# Supplementary material for: Mapping the Global South: Equal-Area Projections for Choropleth Maps
Source: arXiv:2008.13592 ancillary file (2020-09-06)
Supplement: Supplementary file 1 [file maps.pdf]

# Supplemental Material: Maps

In this document, we present the maps created by the social science researchers. Every researcher created two maps: Map 1 for Task 1 and Map 2 for Task 2. Each page contains a section with the maps created by one participant. We specify the map projection in the figure's caption.

## 1 Participant 1

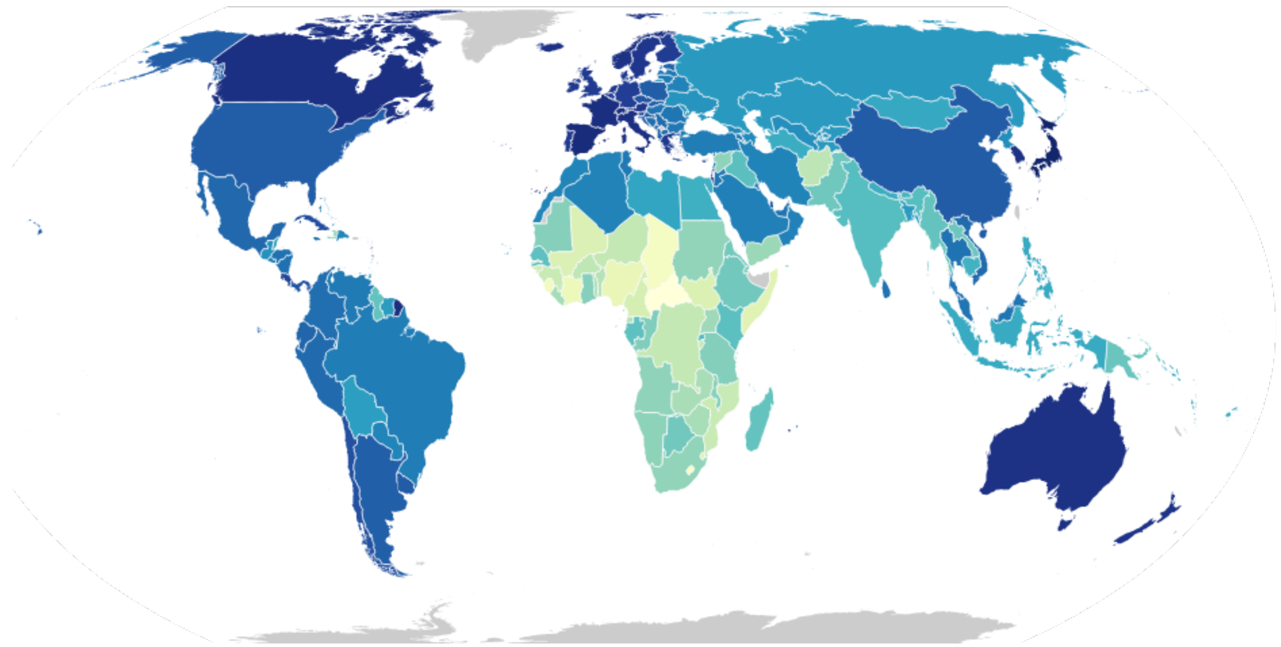

Figure 1: Map 1 of P1. Projection: Equal Earth.

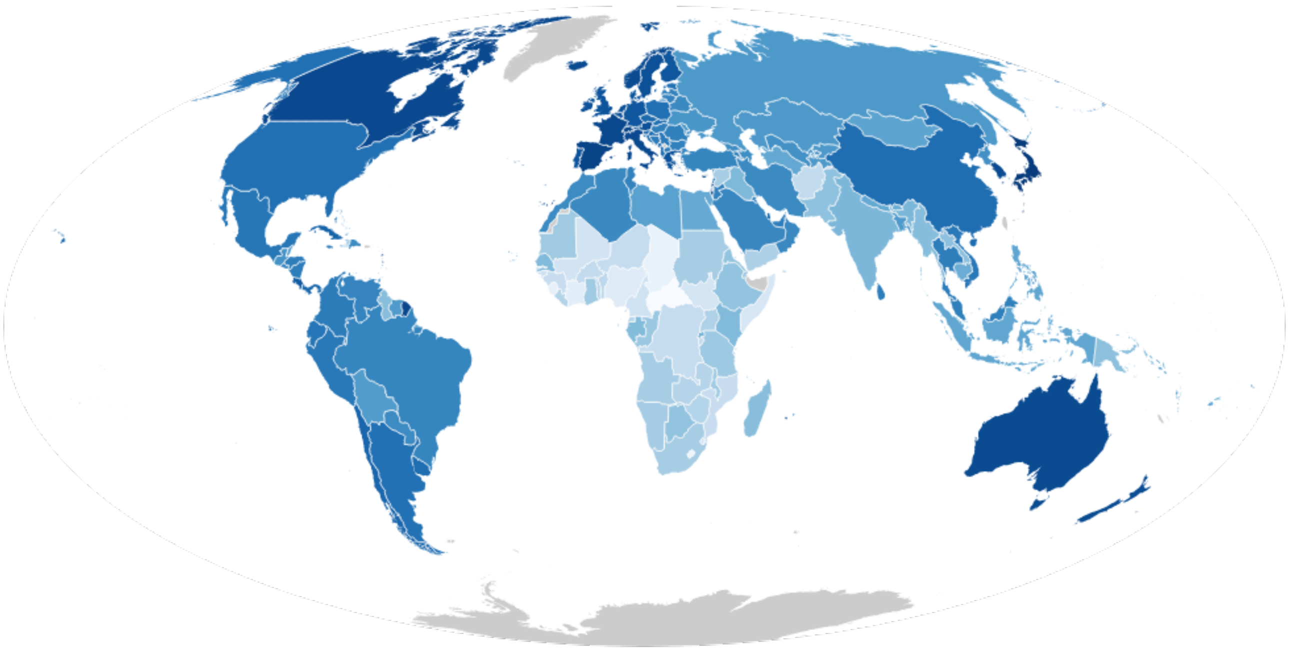

Figure 2: Map 2 of P1. Projection: Mollweide.

## 2 Participant 2

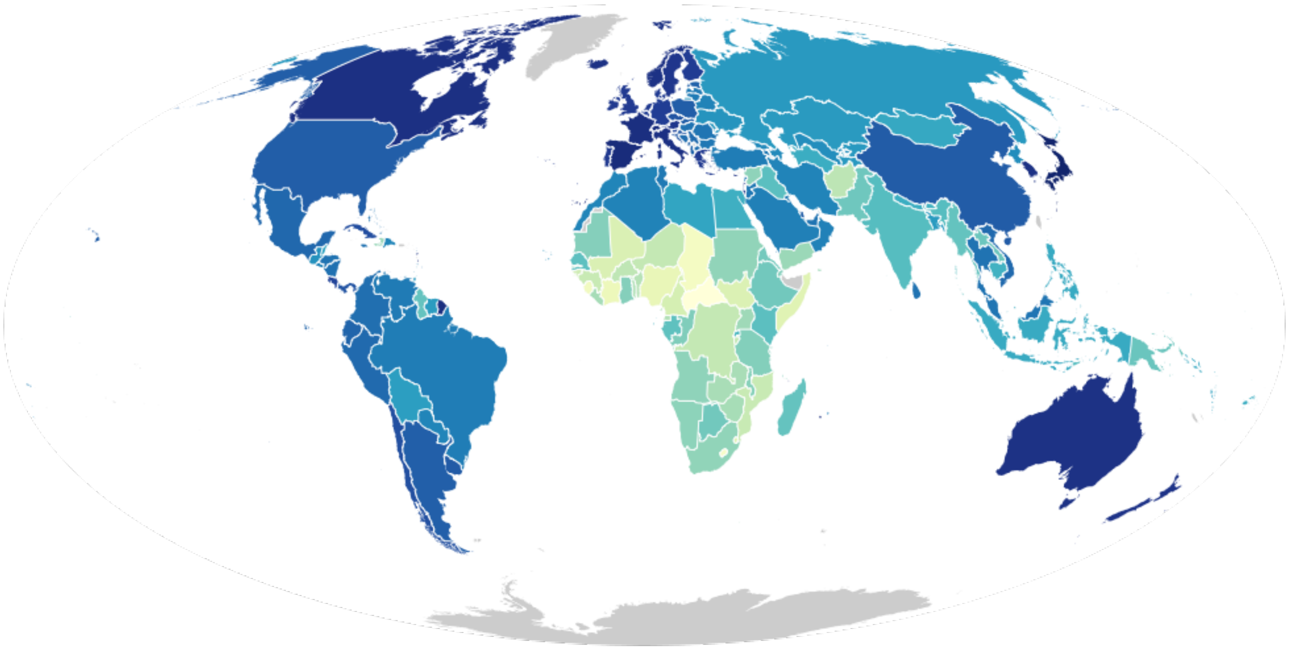

Figure 3: Map 1 of P2. Projection: Mollweide.

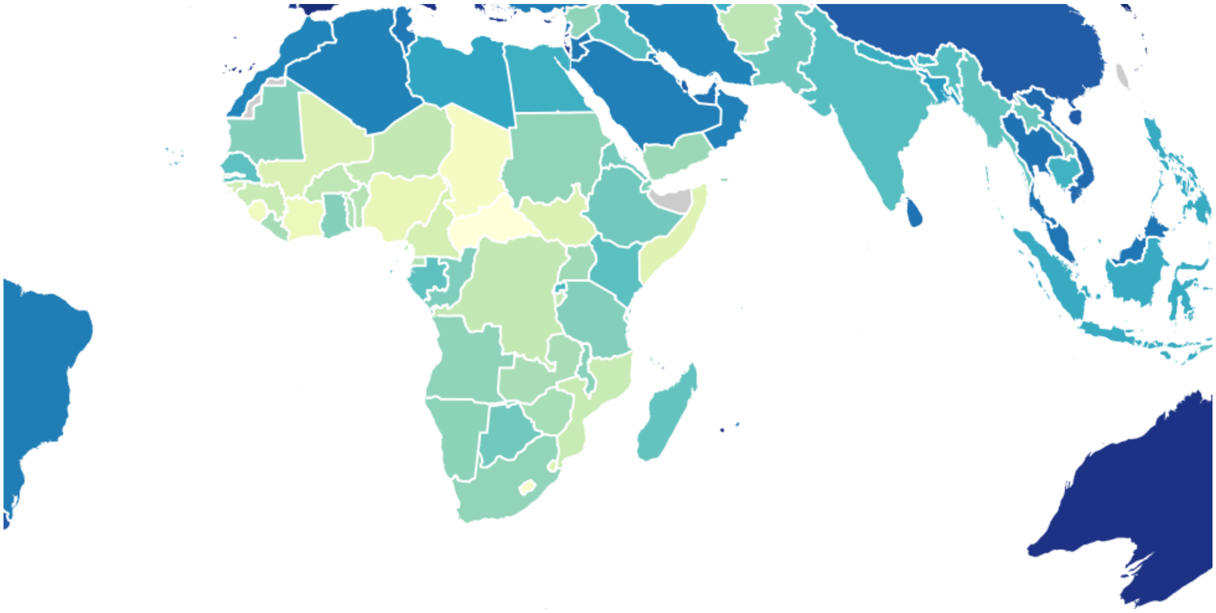

Figure 4: Map 2 of P1. Projection: Hammer.

## 3 Participant 3

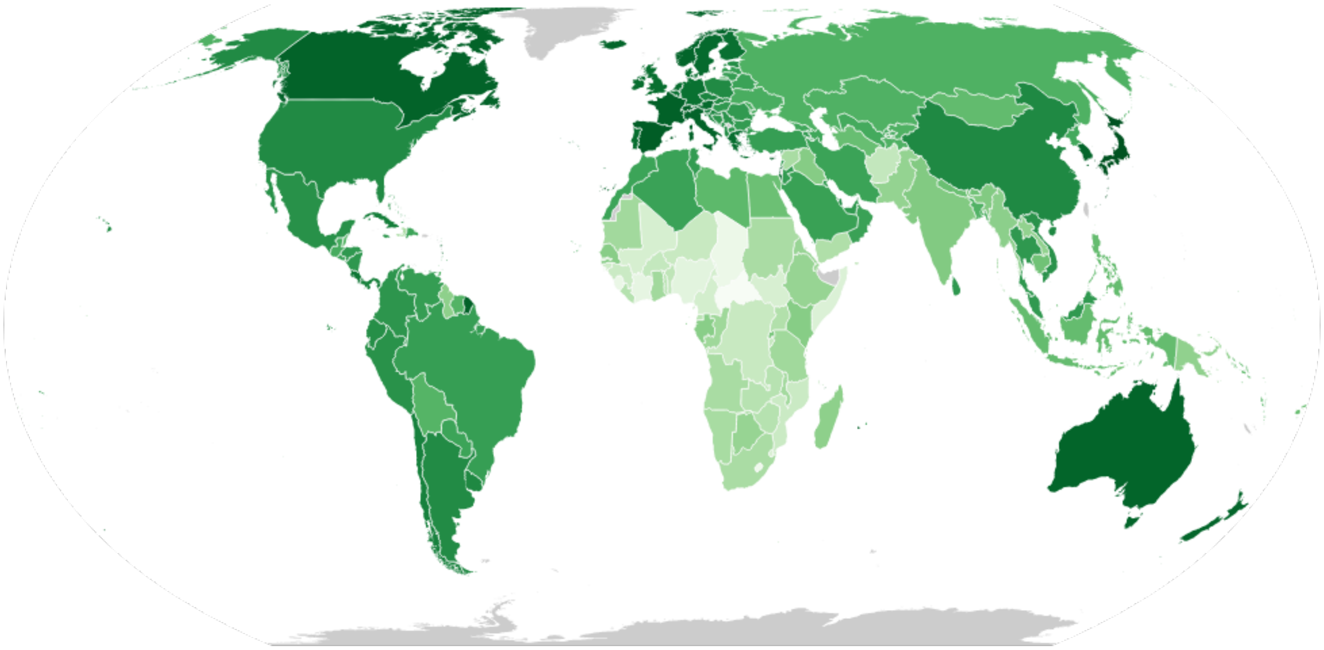

Figure 5: Map 1 of P3. Projection: Equal Earth.

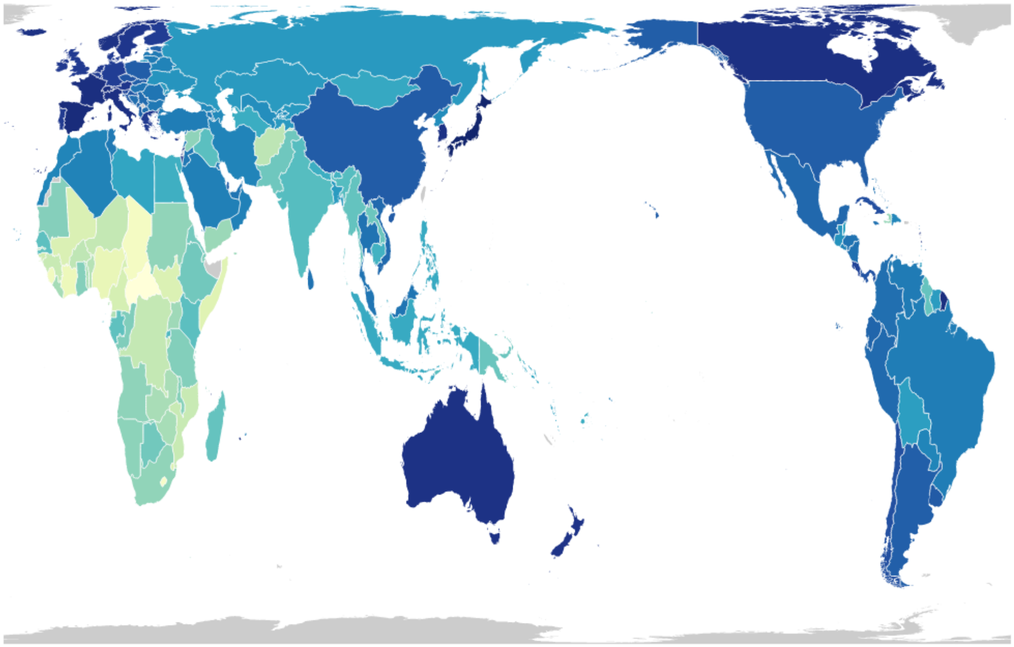

Figure 6: Map 2 of P3. Projection: Gall-Peters.

## 4 PARTICIPANT 4

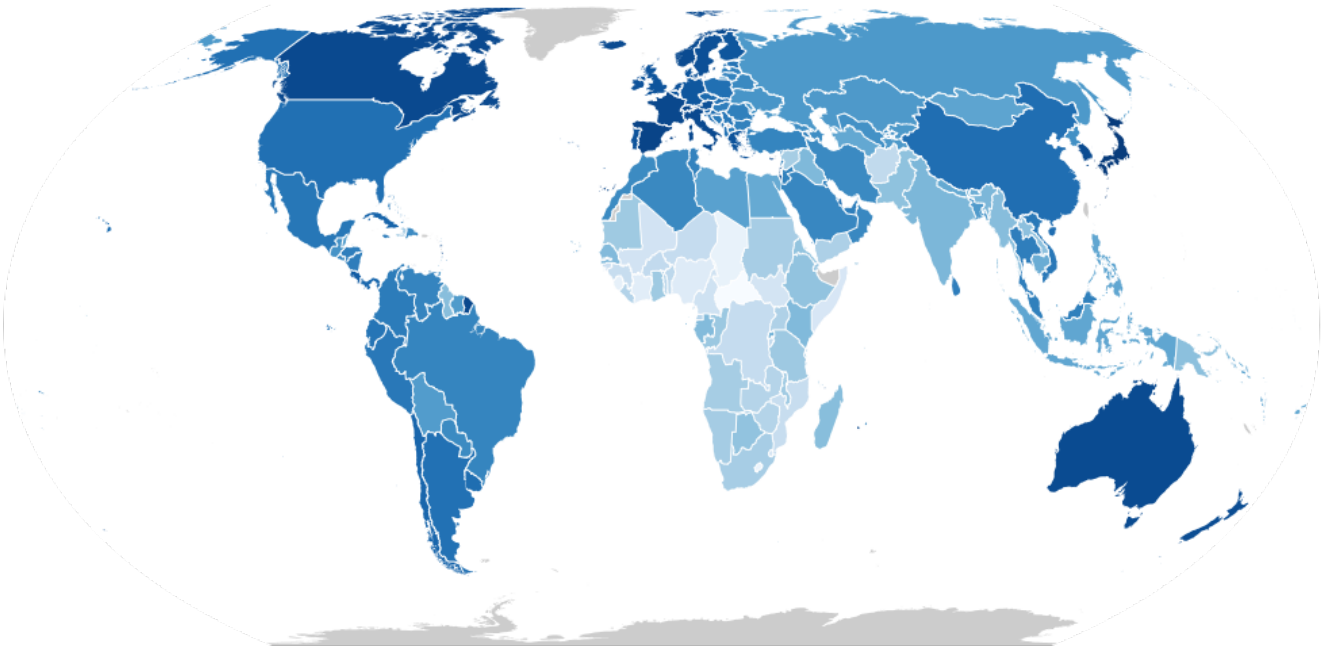

Figure 7: Map 1 of P4. Projection: Equal Earth.

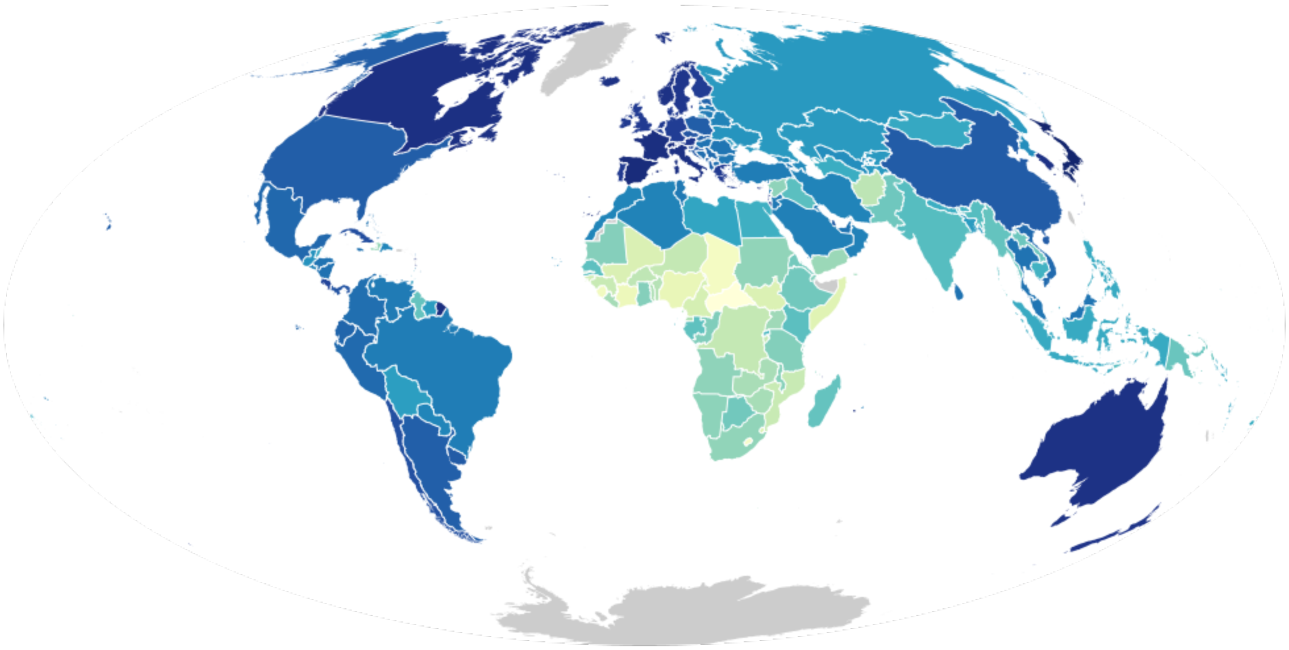

Figure 8: Map 2 of P4. Projection: Hammer.

## 5 PARTICIPANT 5

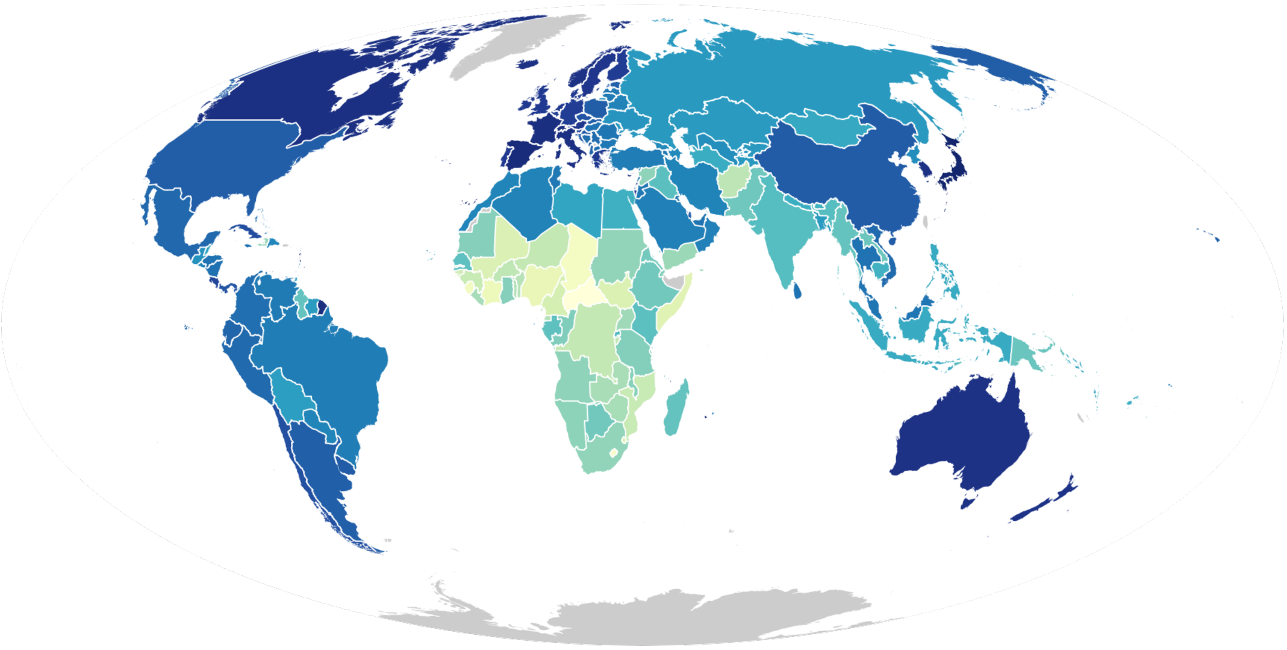

Figure 9: Map 1 of P5. Projection: Mollweide.

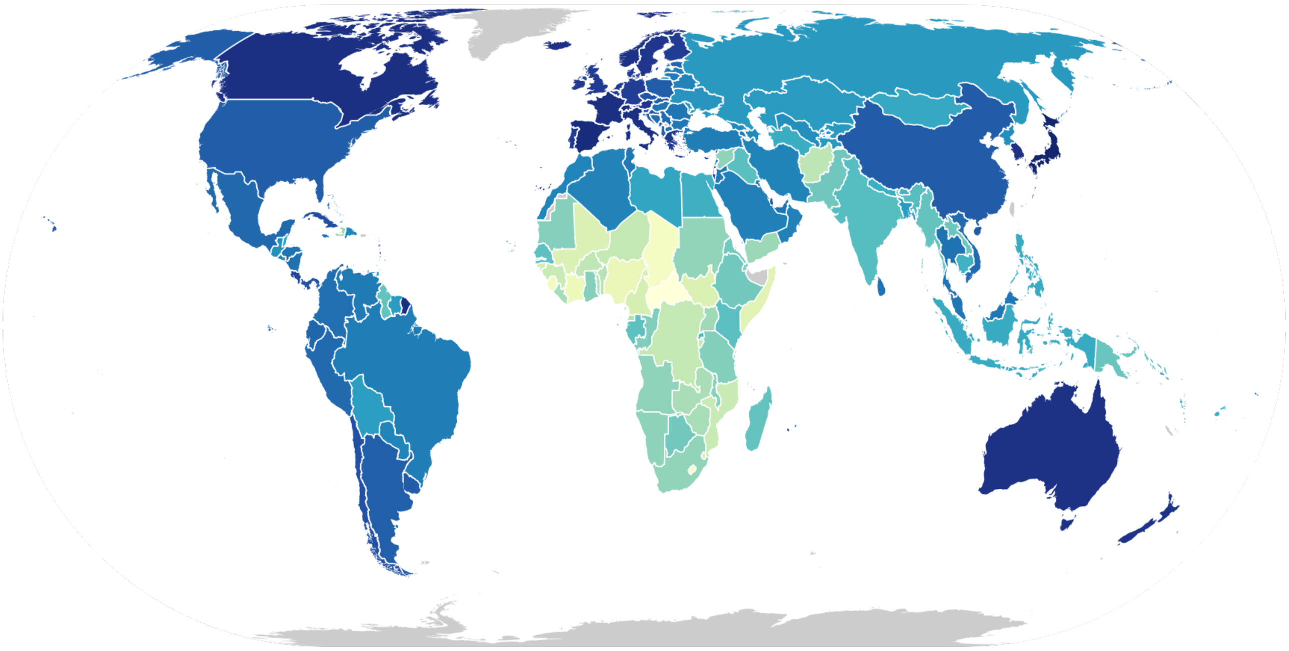

Figure 10: Map 2 of P5. Projection: Eckert IV.

## 6 Participant 6

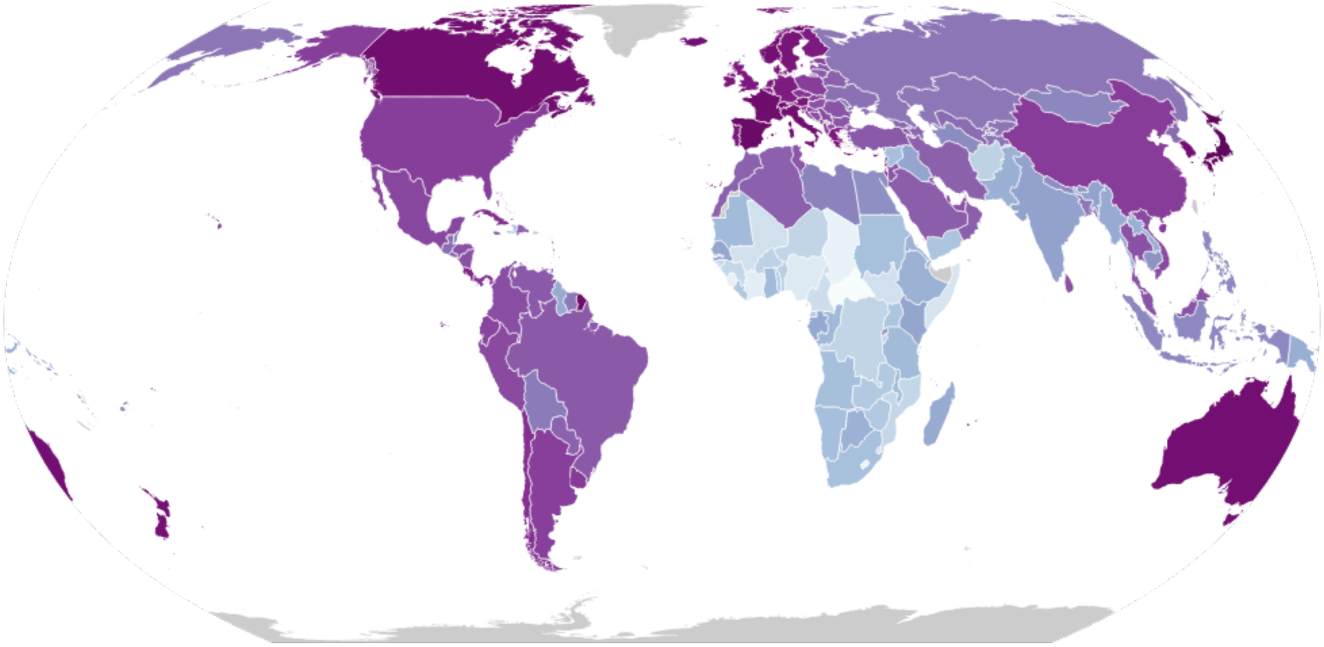

Figure 11: Map 1 of P6. Projection: Equal Earth.

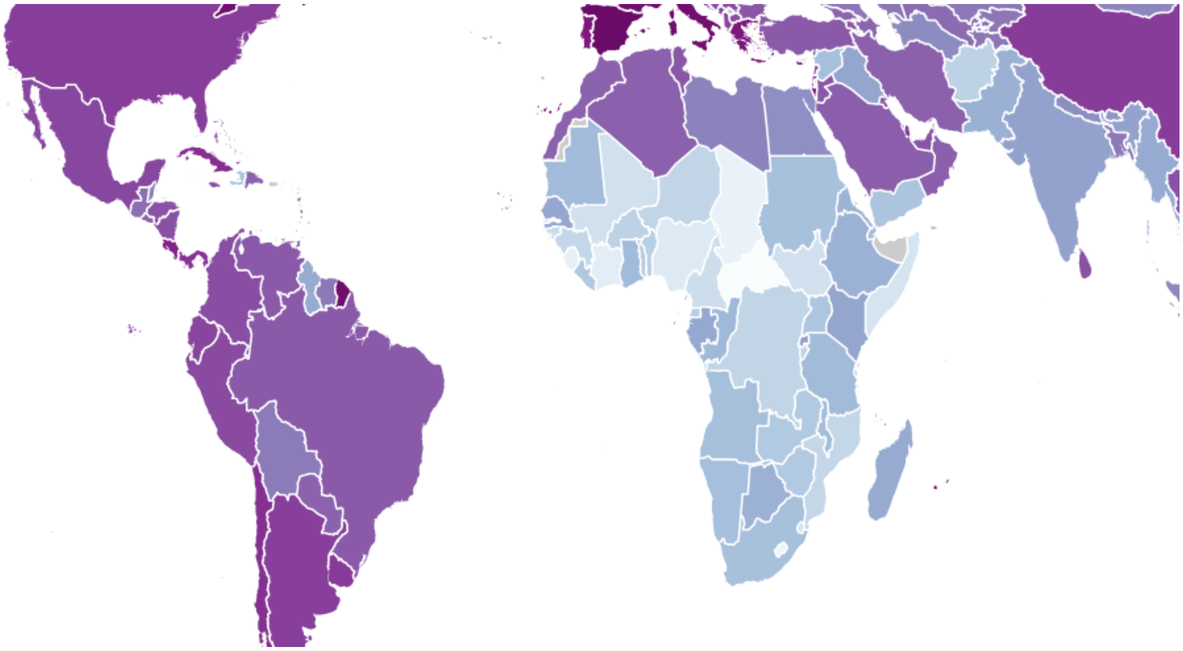

Figure 12: Map 2 of P6. Projection: Eckert IV.

## 7 PARTICIPANT 7

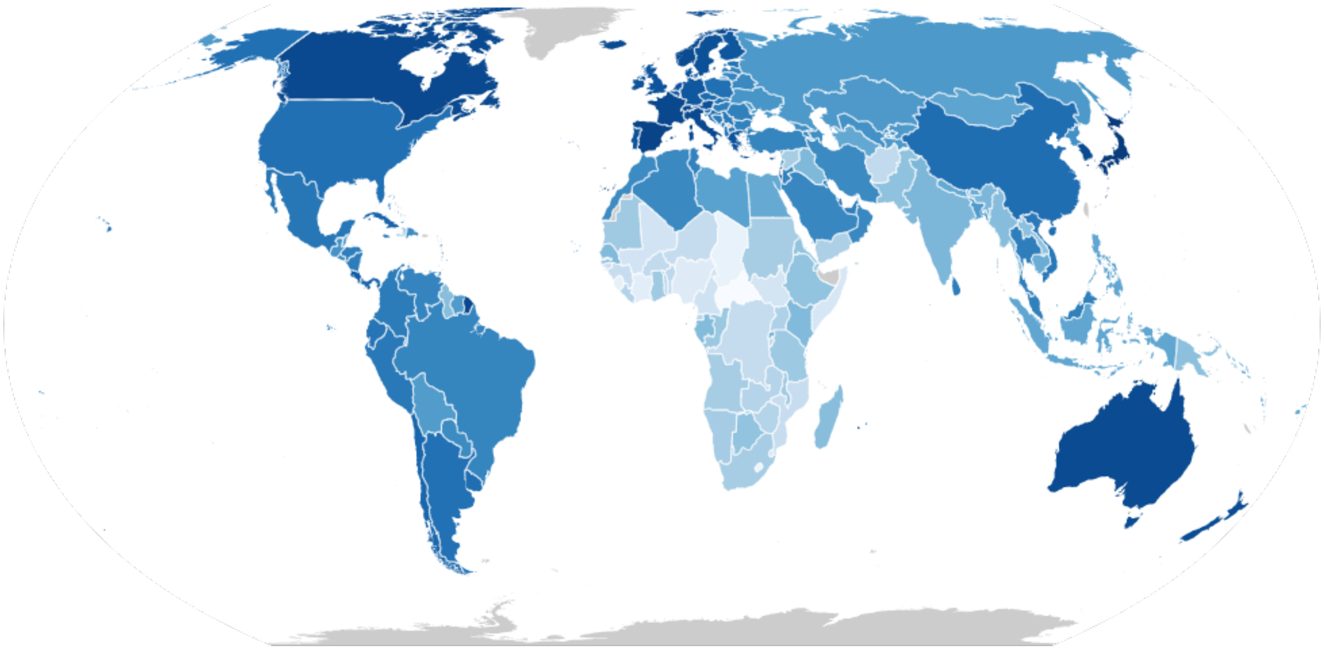

Figure 13: Map 1 of P7. Projection: Equal Earth.

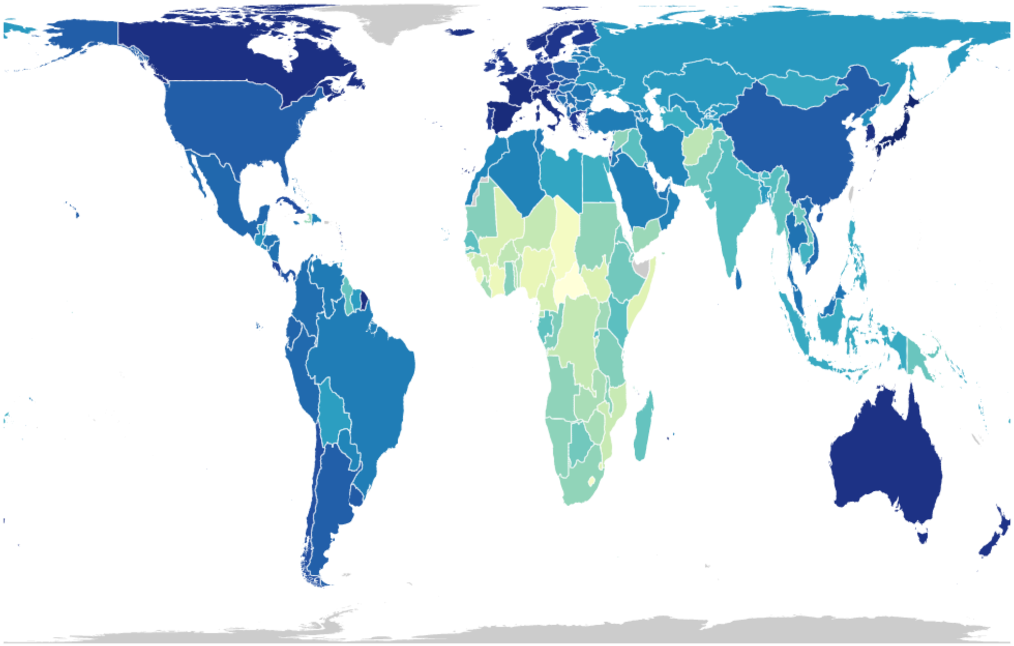

Figure 14: Map 2 of P7. Projection: Gall-Peters.

## 8 PARTICIPANT 8

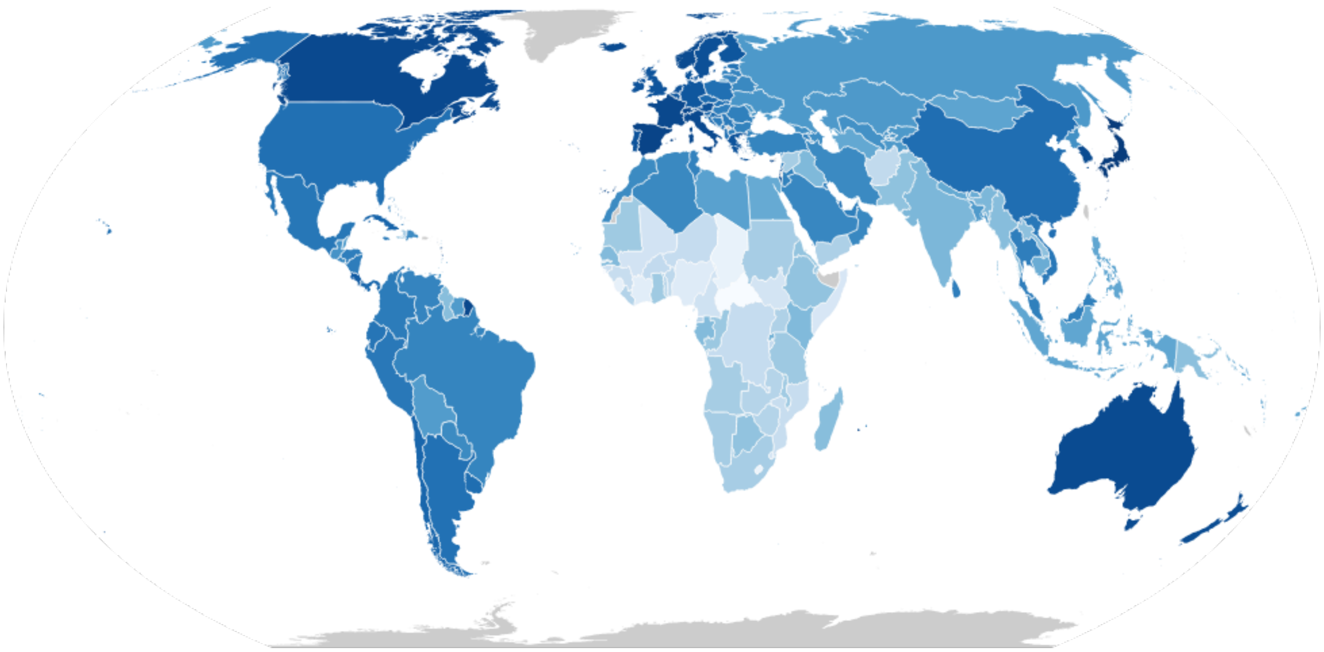

Figure 15: Map 1 of P8. Projection: Equal Earth.

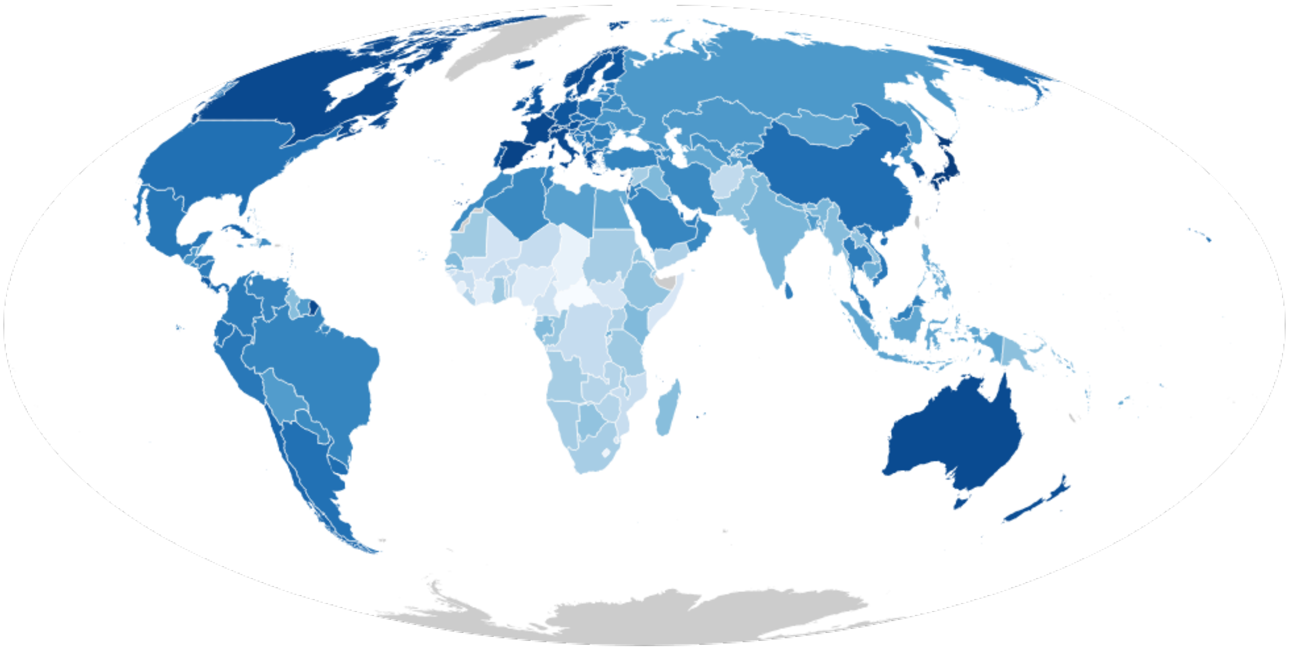

Figure 16: Map 2 of P8. Projection: Mollweide.

## 9 PARTICIPANT 9

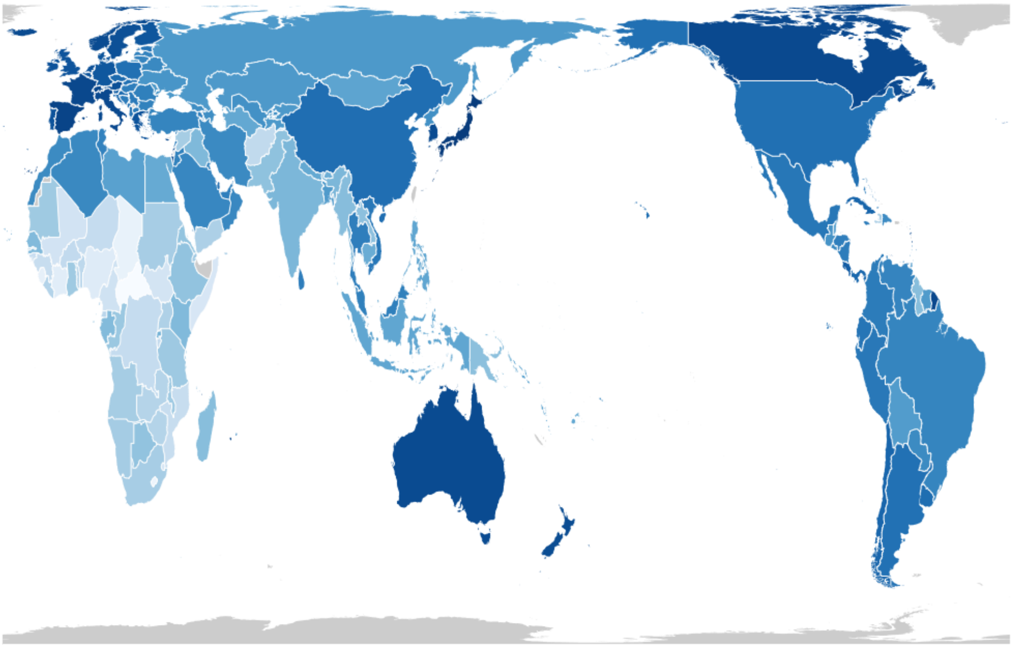

Figure 17: Map 1 of P9. Projection: Gall-Peters.

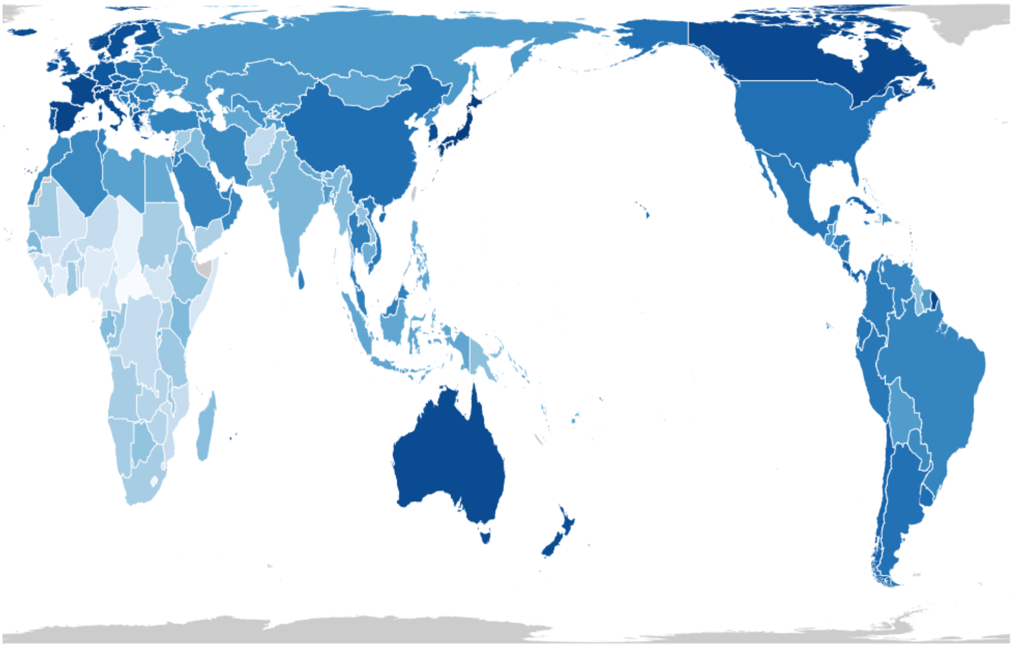

Figure 18: Map 2 of P9. Projection: Gall-Peters.

## 10 Participant 10

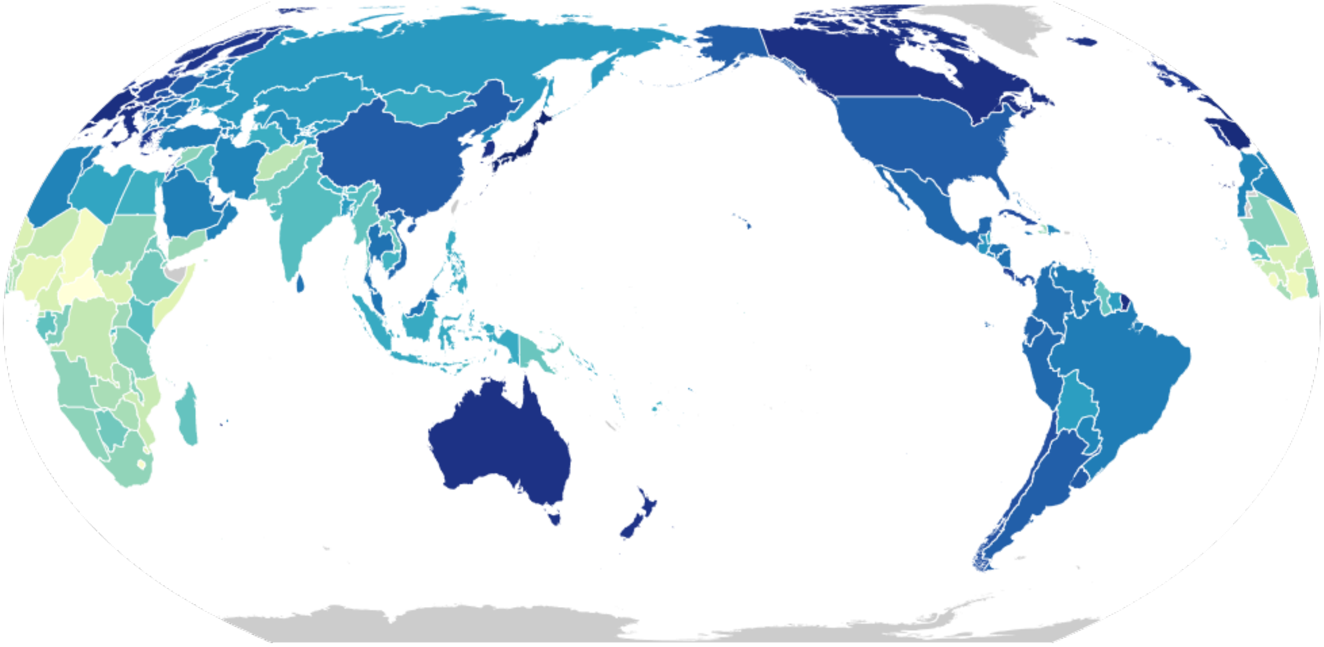

Figure 19: Map 1 of P10. Projection: Equal-Earth.

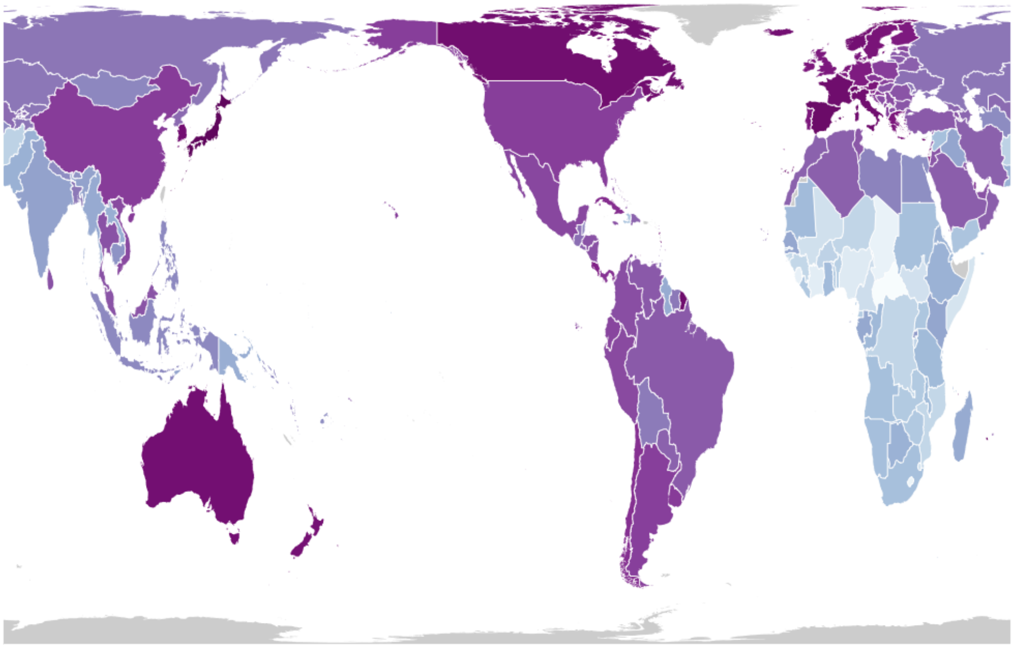

Figure 20: Map 2 of P10. Projection: Gall-Peters.

## 11 PARTICIPANT 11

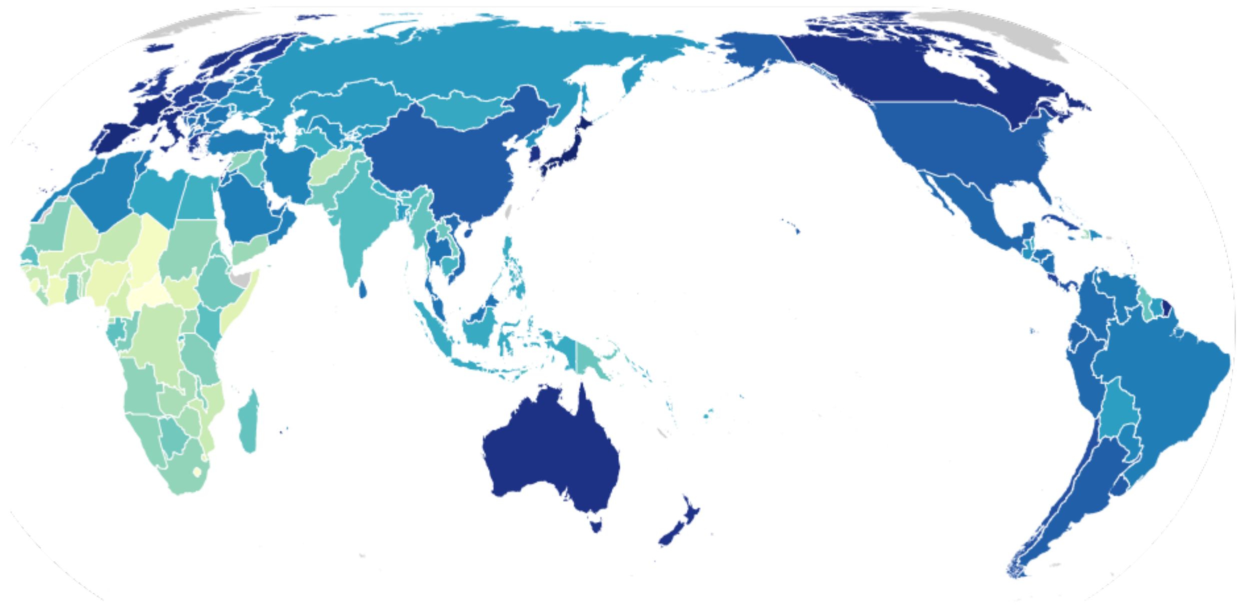

Figure 21: Map 1 of P11. Projection: Eckert IV.

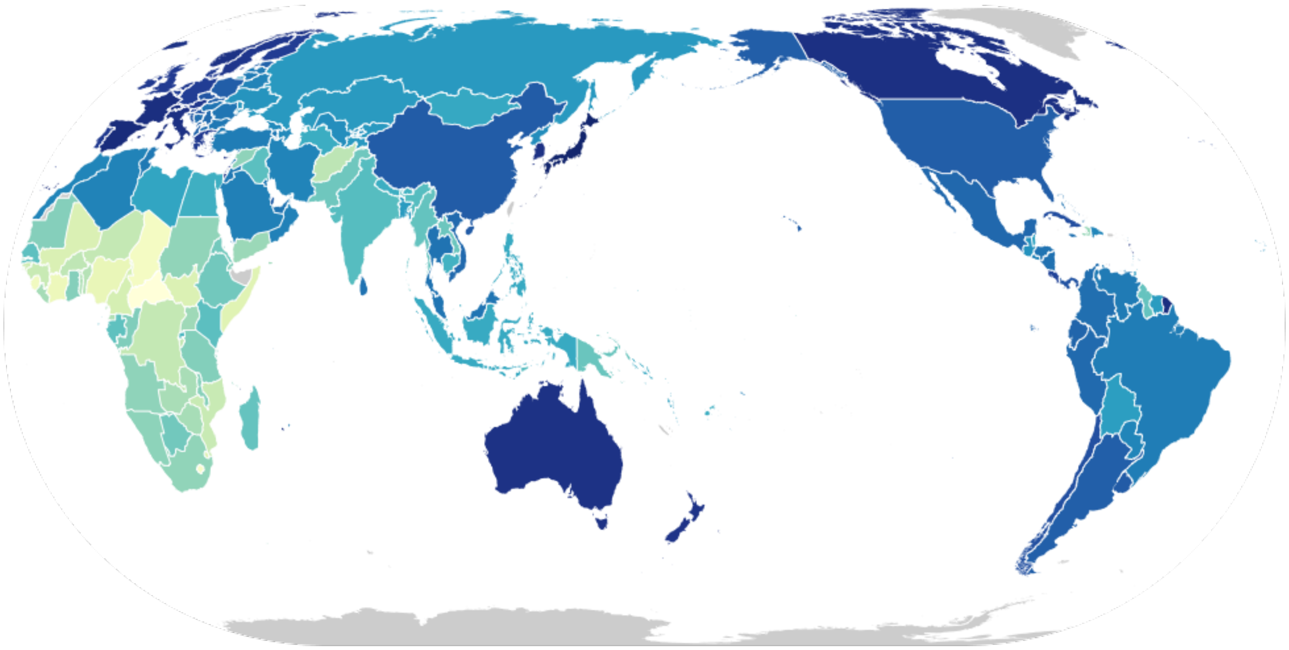

Figure 22: Map 2 of P11. Projection: Eckert IV.

## 12 Participant 12

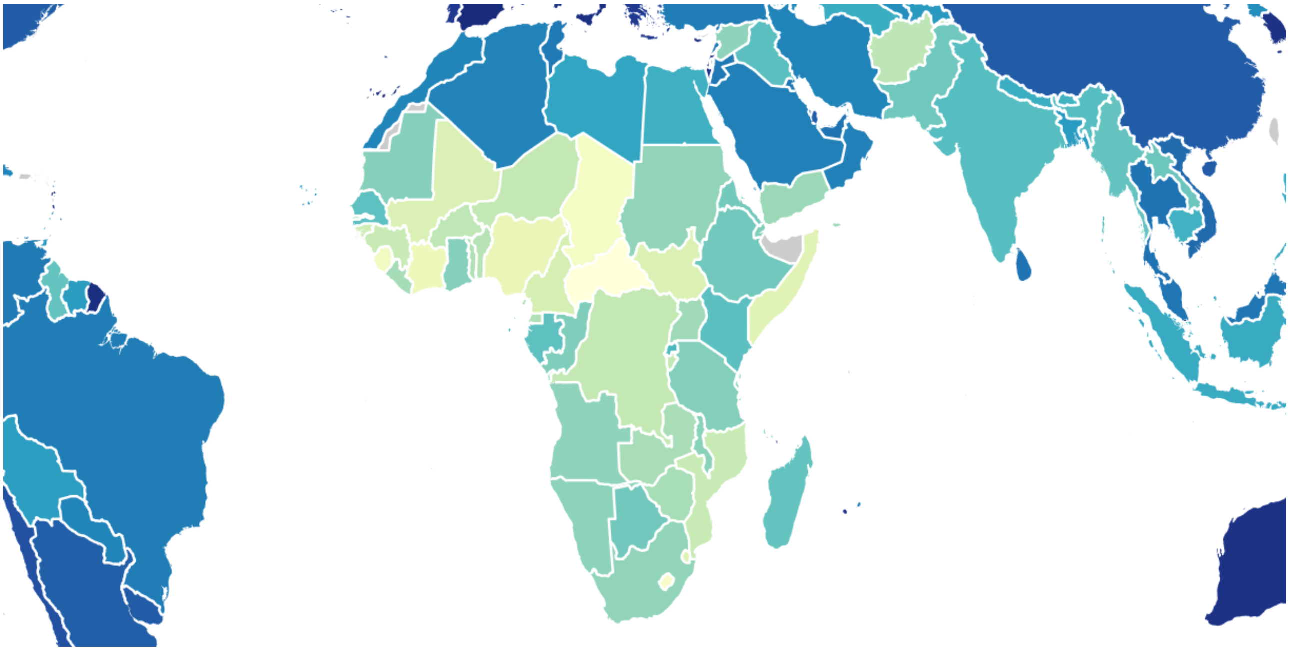

Figure 23: Map 1 of P12. Projection: Mollweide.

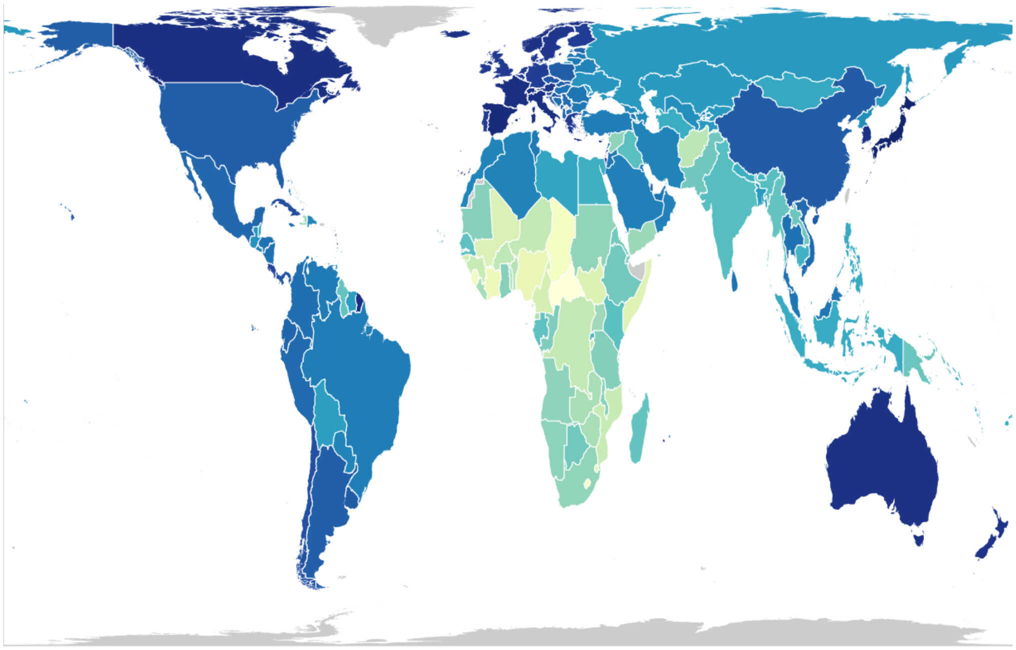

Figure 24: Map 2 of P12. Projection: Gall-Peters.

## 13 Participant 13

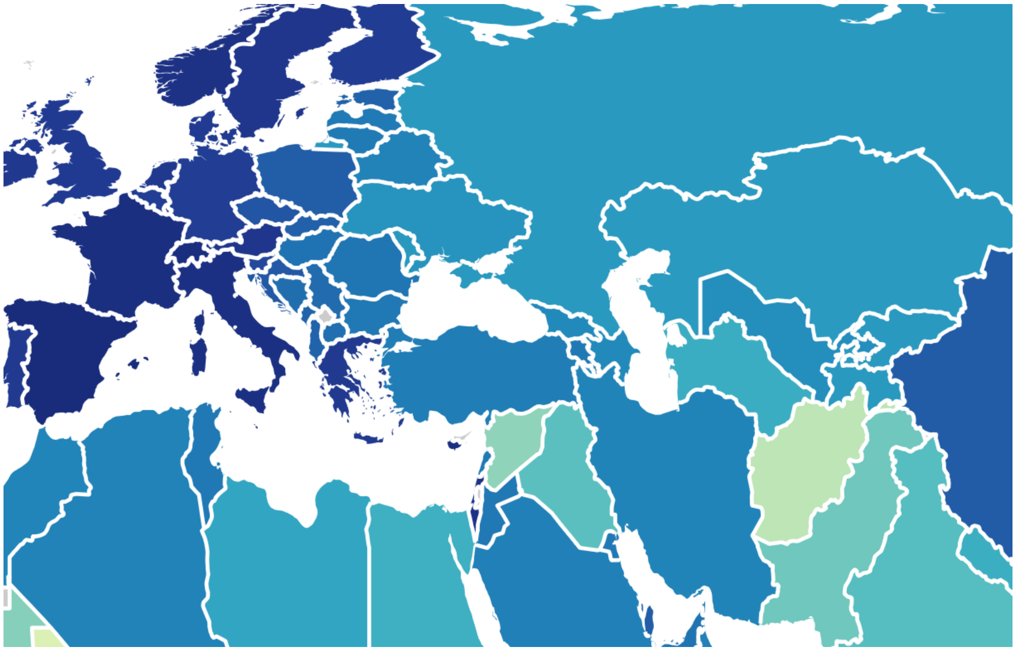

Figure 25: Map 1 of P13. Projection: Gall-Peters.

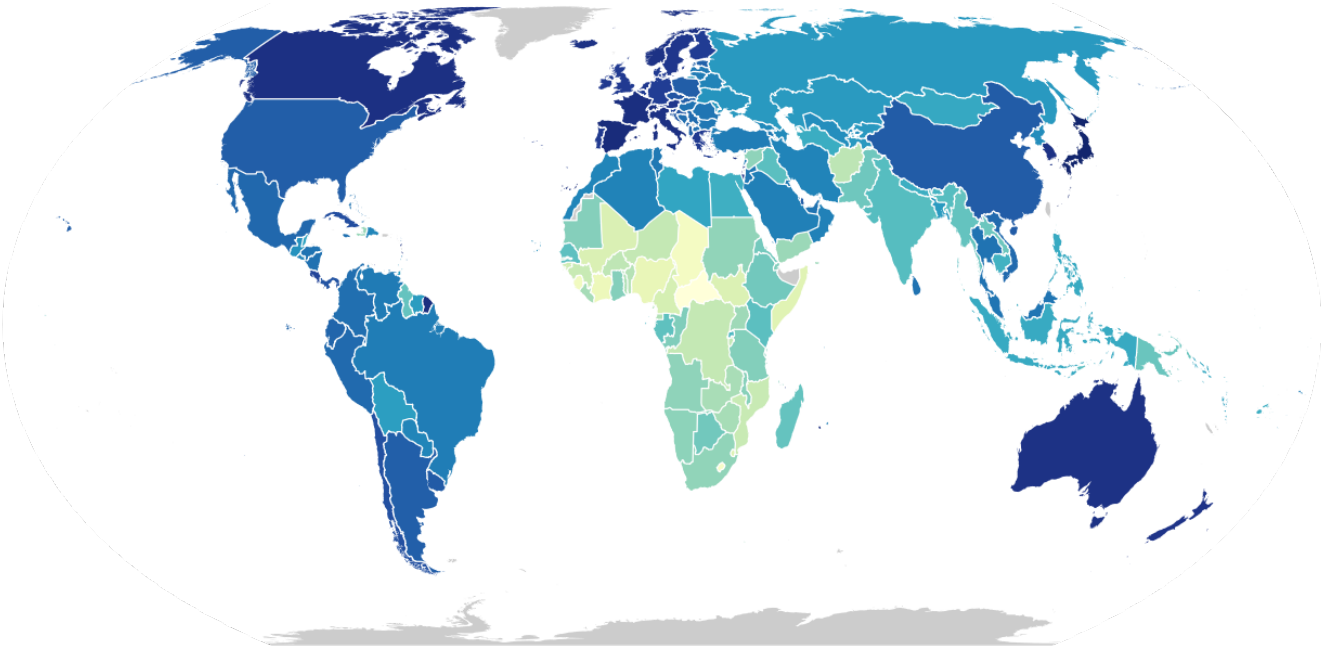

Figure 26: Map 2 of P13. Projection: Equal Earth.

## 14 Participant 14

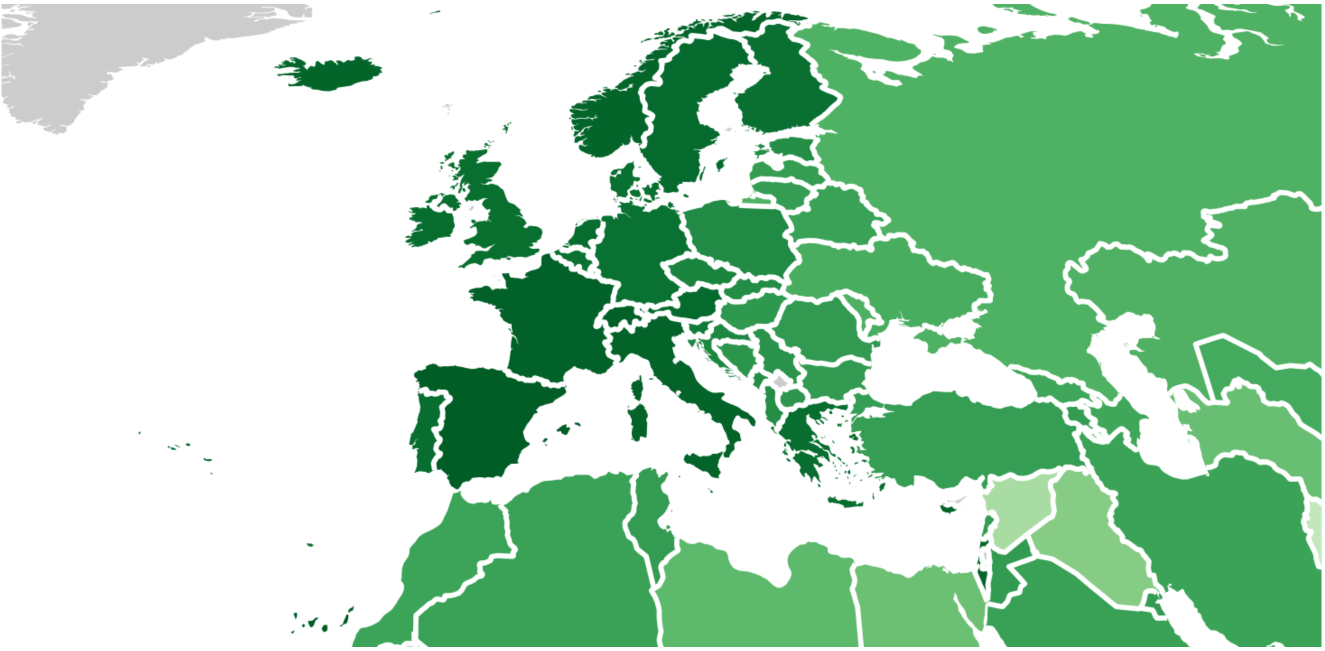

Figure 27: Map 1 of P14. Projection: Equal Earth.

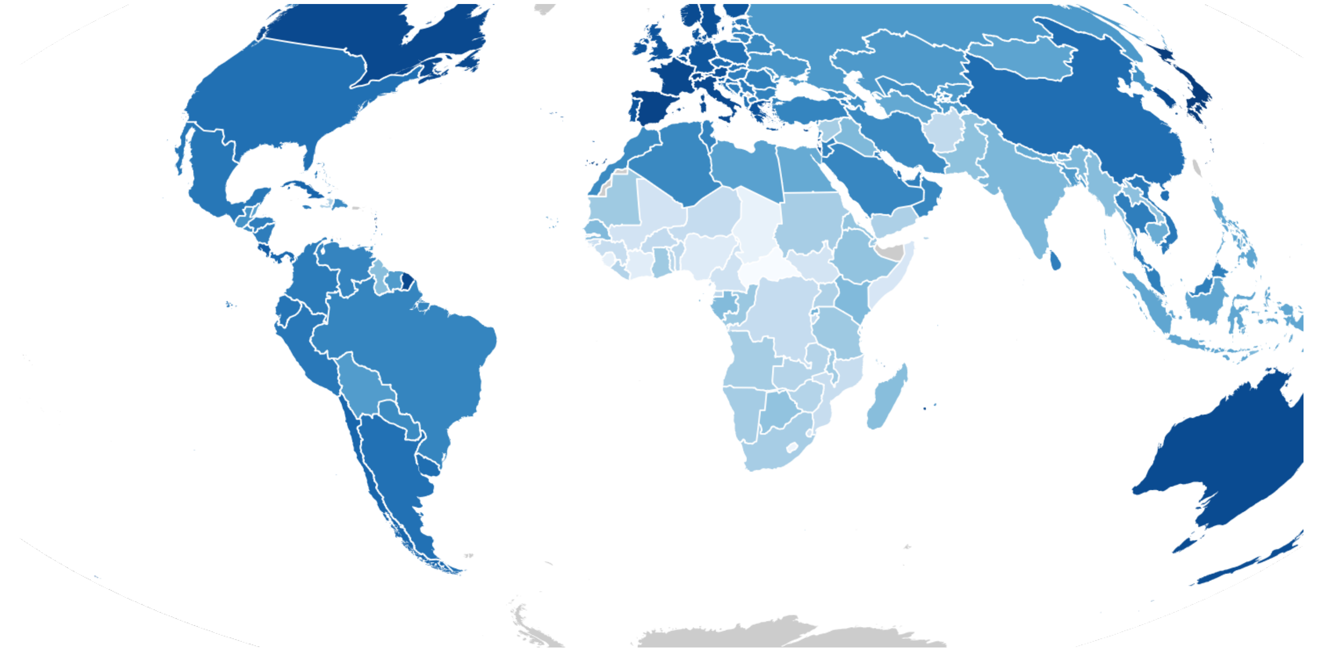

Figure 28: Map 2 of P14. Projection: Hammer.

## 15 Participant 15

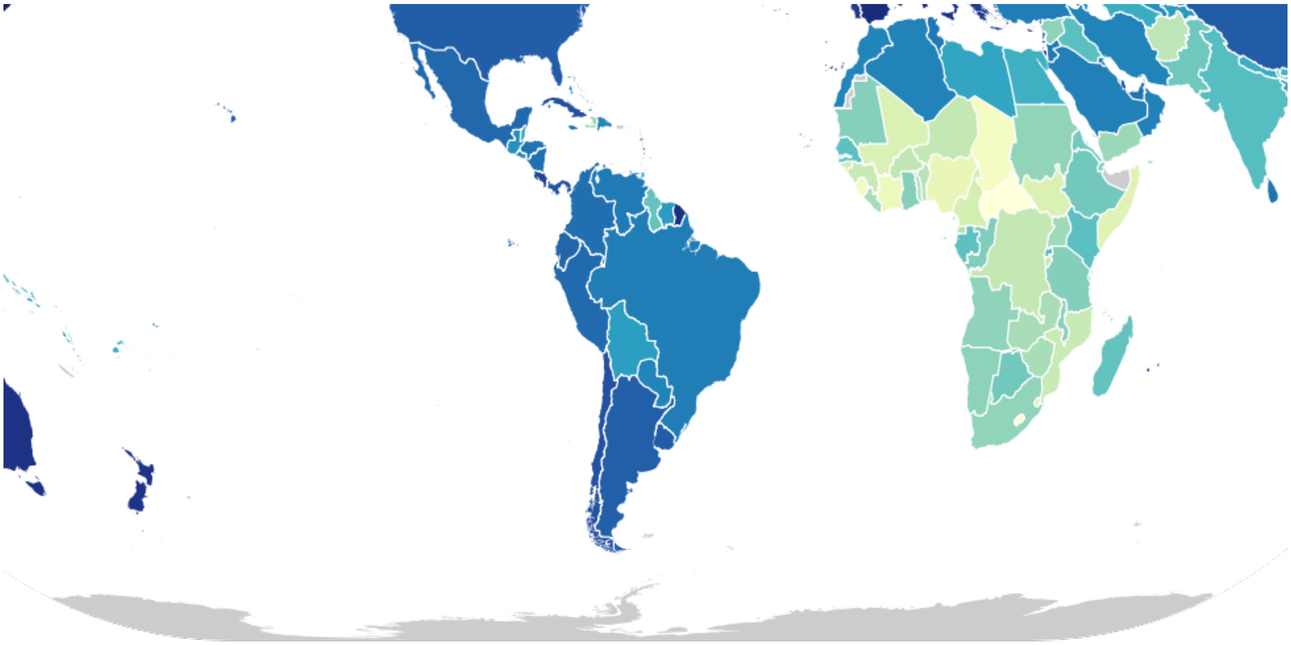

Figure 29: Map 1 of P15. Projection: Eckert IV.

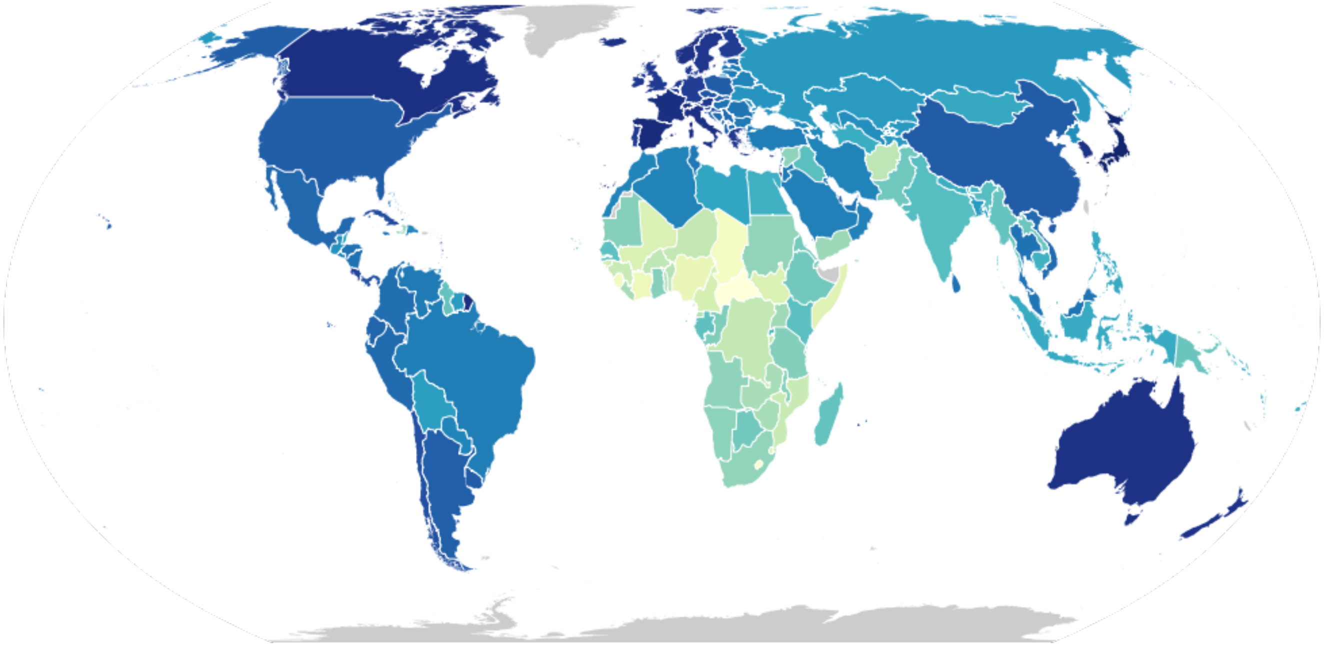

Figure 30: Map 2 of P15. Projection: Equal Earth.

## 16 Participant 16

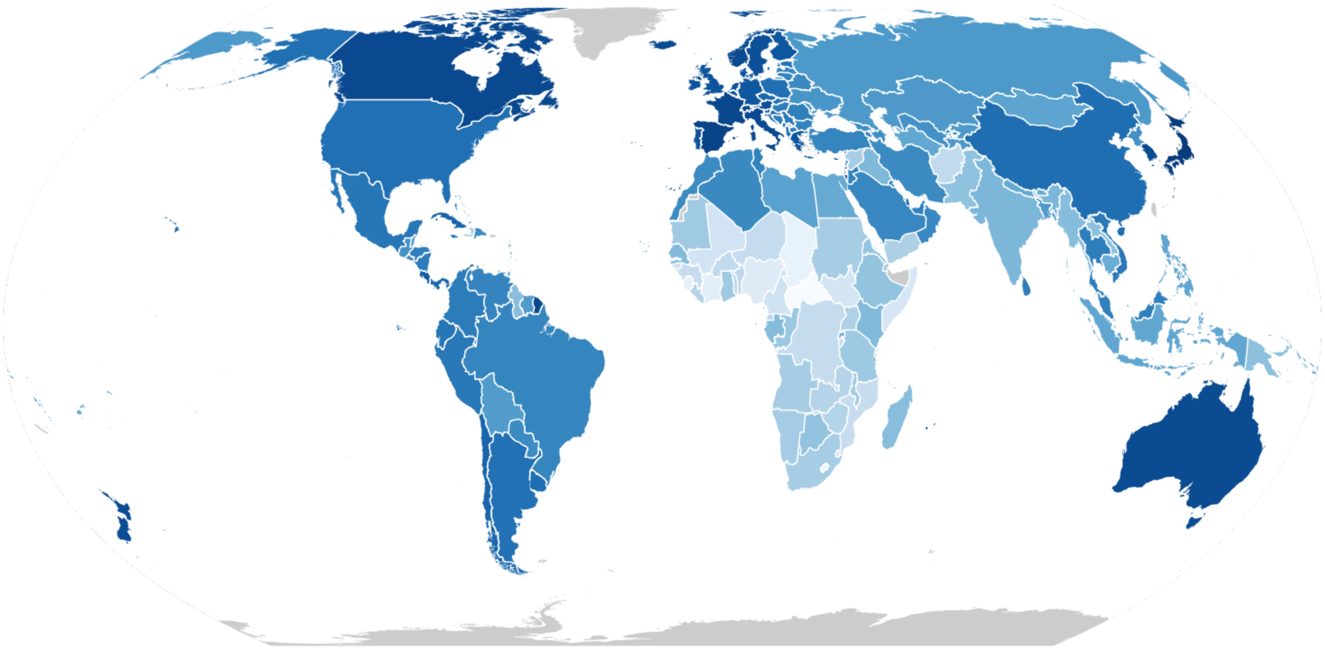

Figure 31: Map 1 of P16. Projection: Equal Earth.

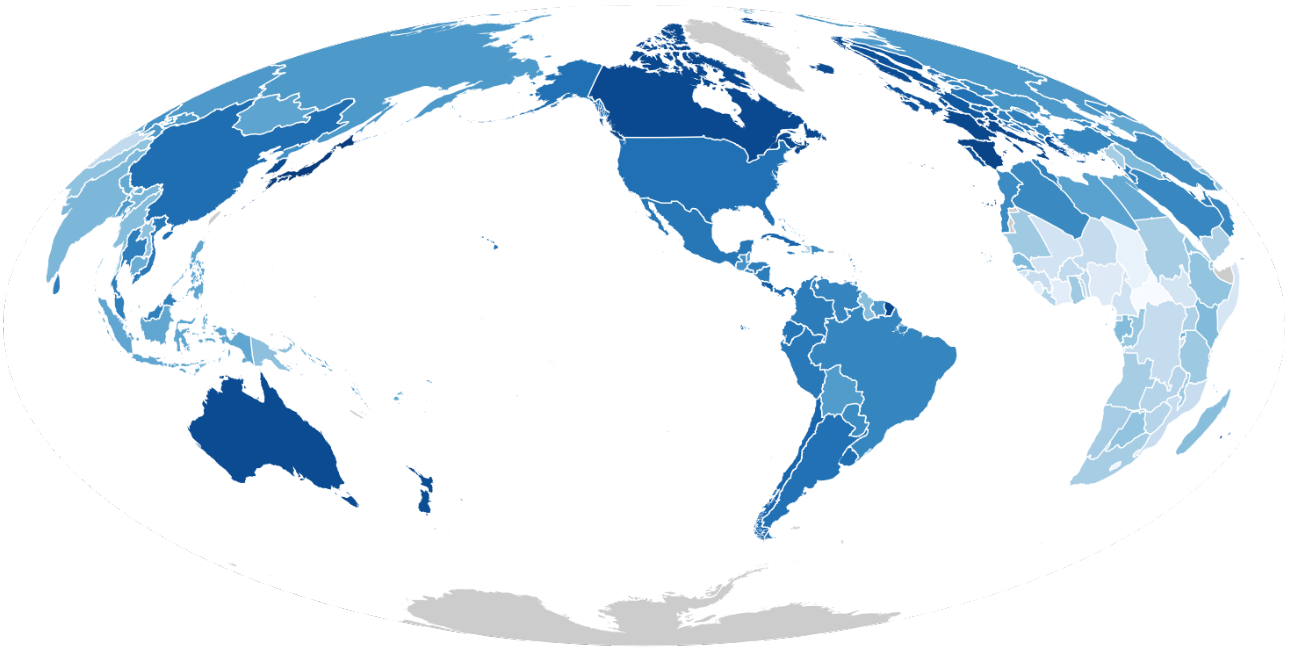

Figure 32: Map 2 of P16. Projection: Hammer.

## 17 PARTICIPANT 17

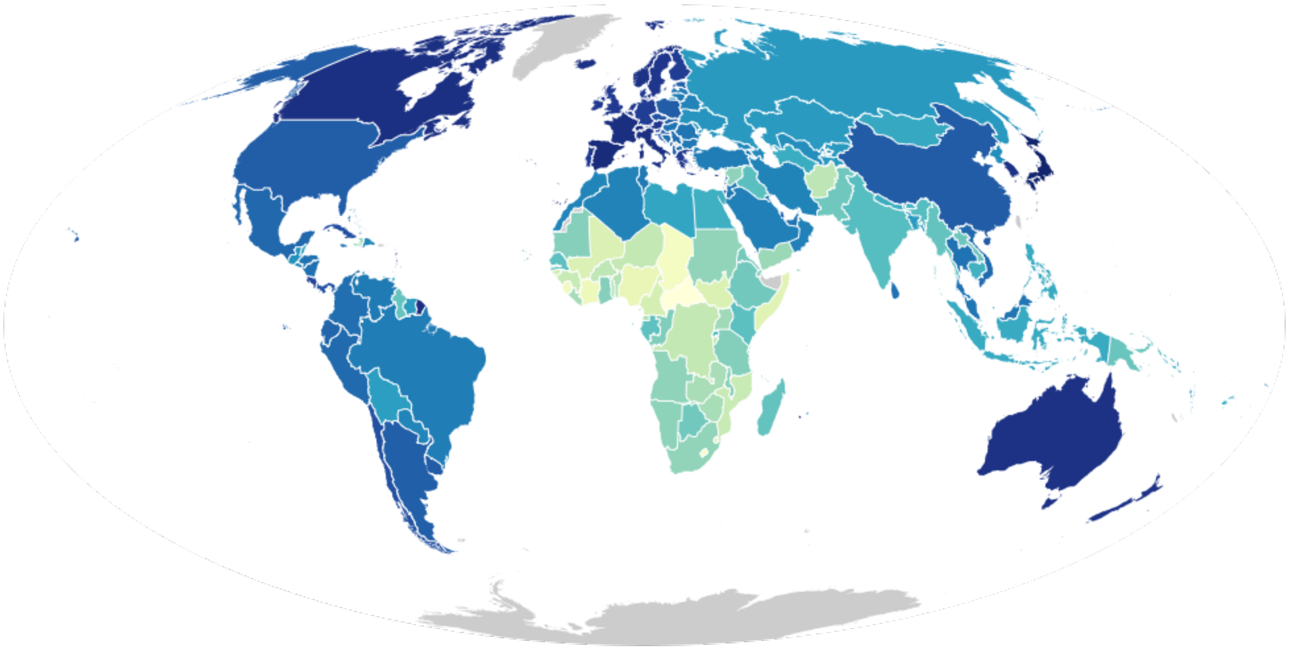

Figure 33: Map 1 of P17. Projection: Mollweide.

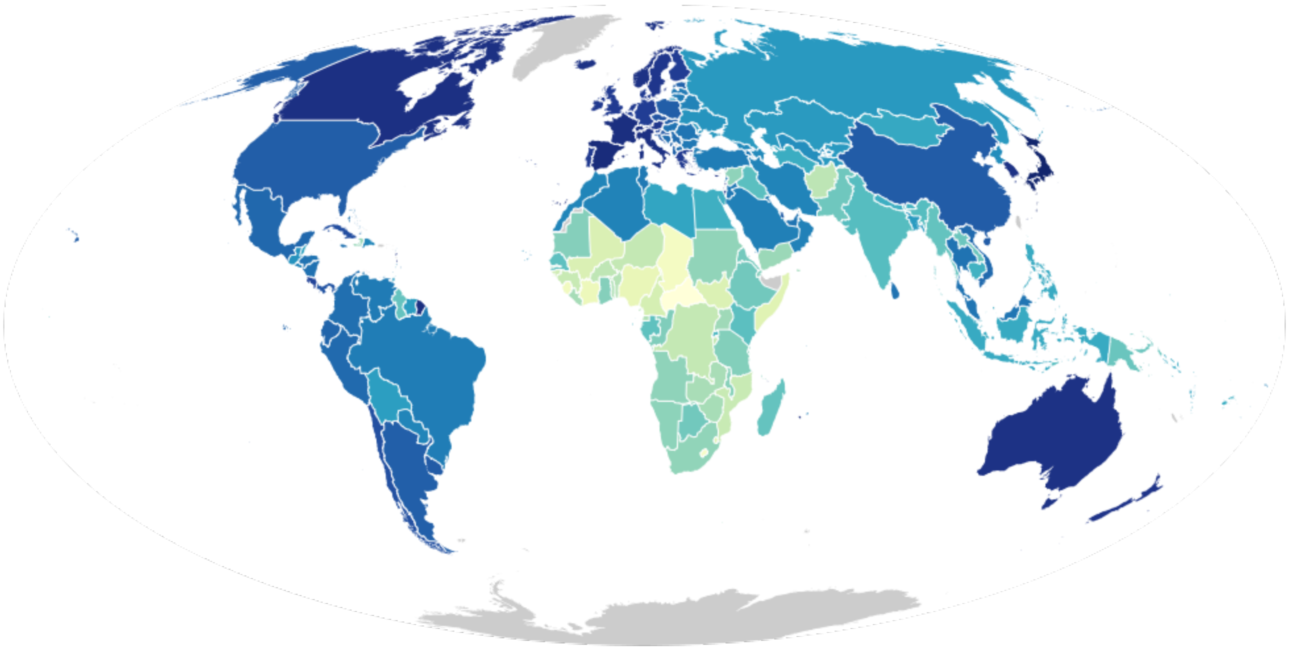

Figure 34: Map 2 of P17. Projection: Mollweide.

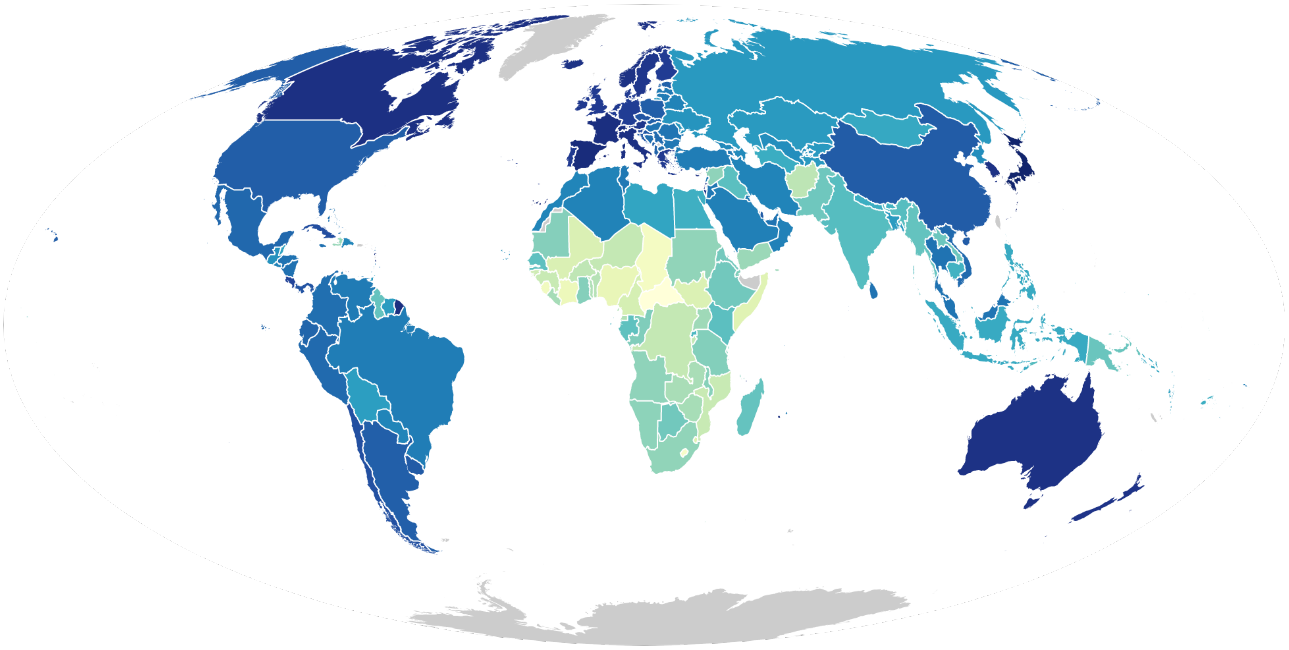

Figure 35: Map 1 of P18. Projection: Mollweide.

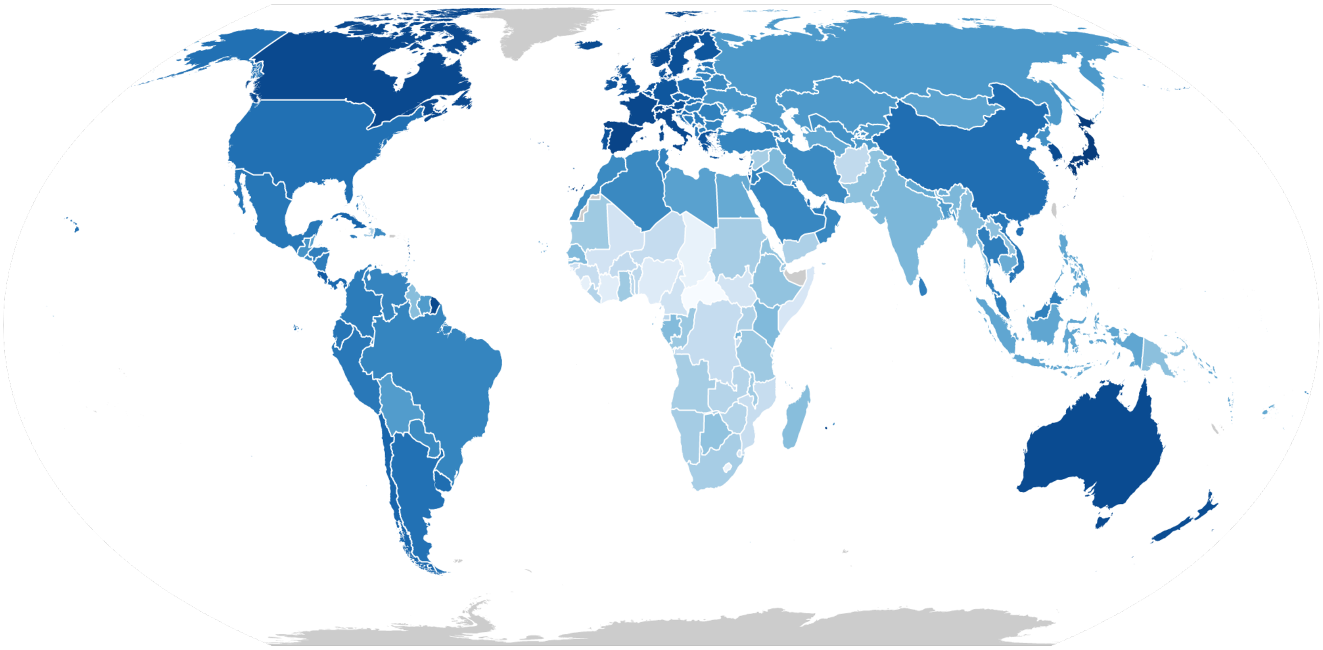

Figure 36: Map 2 of P18. Projection: Equal Earth.

## 19 Participant 19

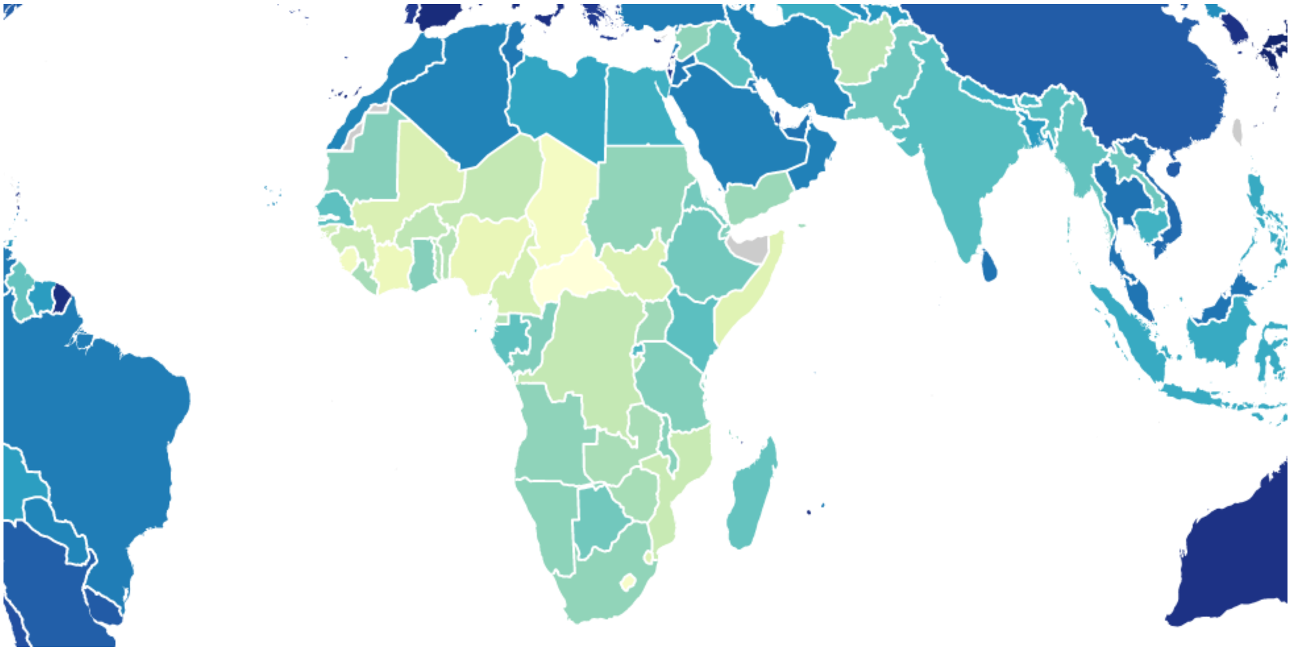

Figure 37: Map 1 of P19. Projection: Mollweide.

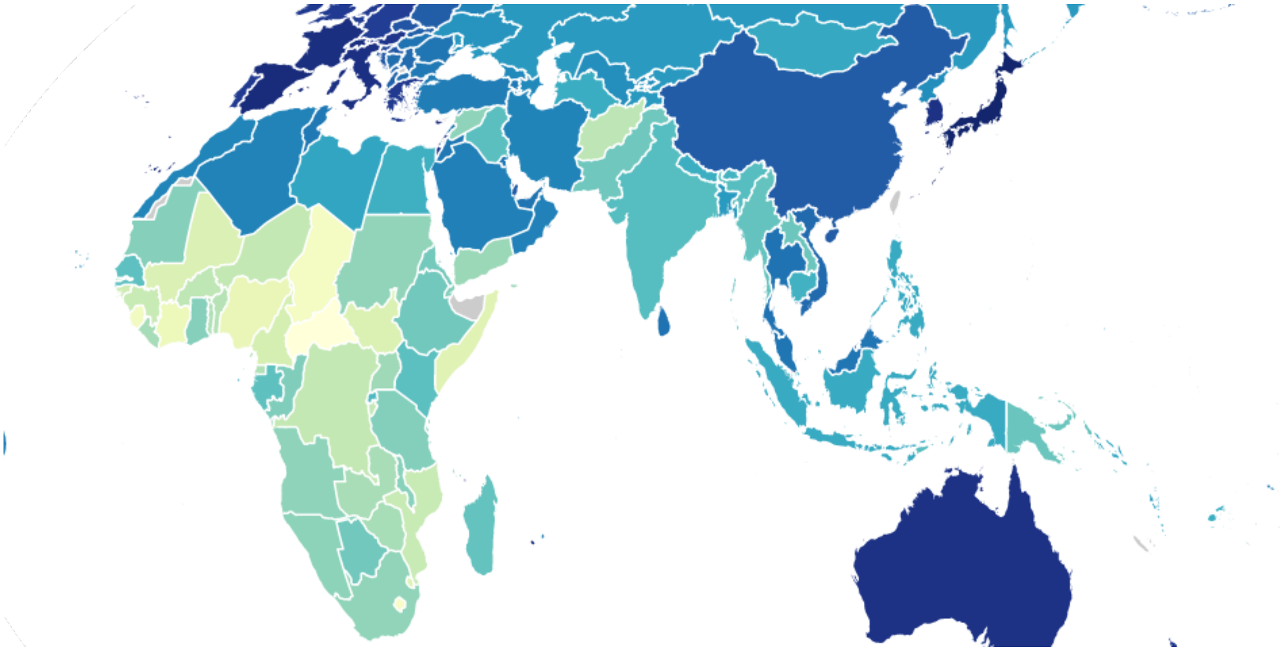

Figure 38: Map 2 of P19. Projection: Equal Earth.

# 20 Participant 20

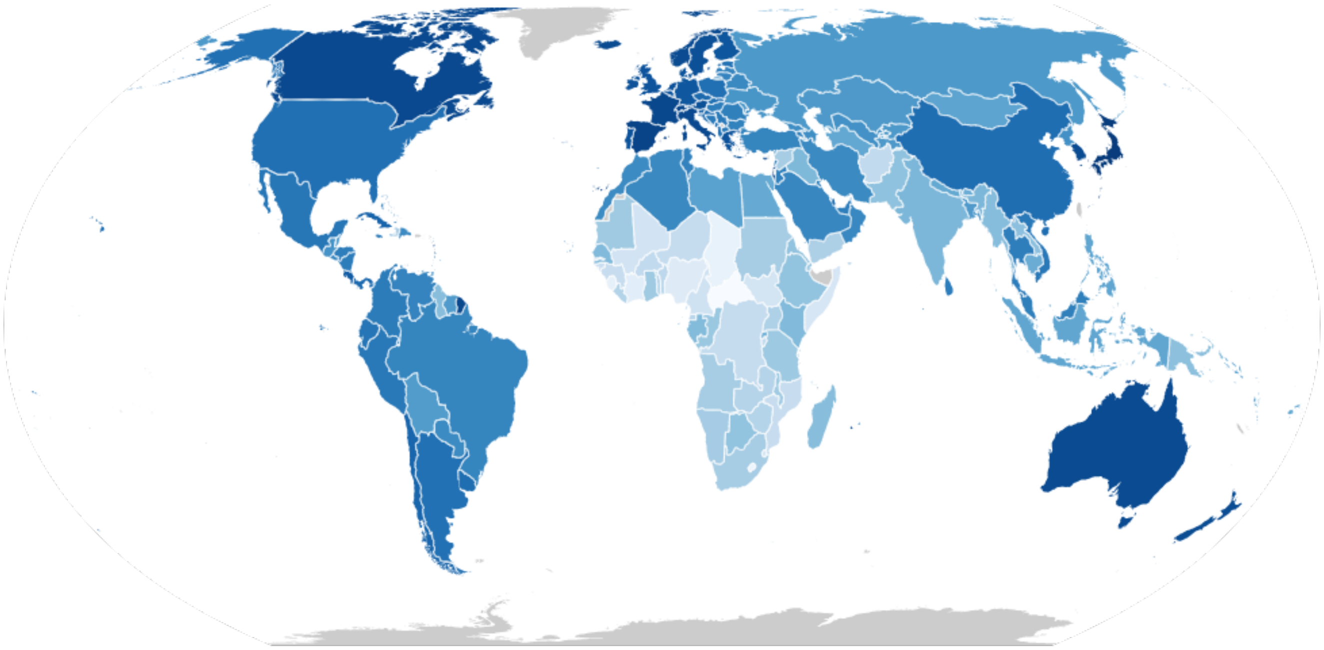

Figure 39: Map 1 of P20. Projection: Equal Earth.

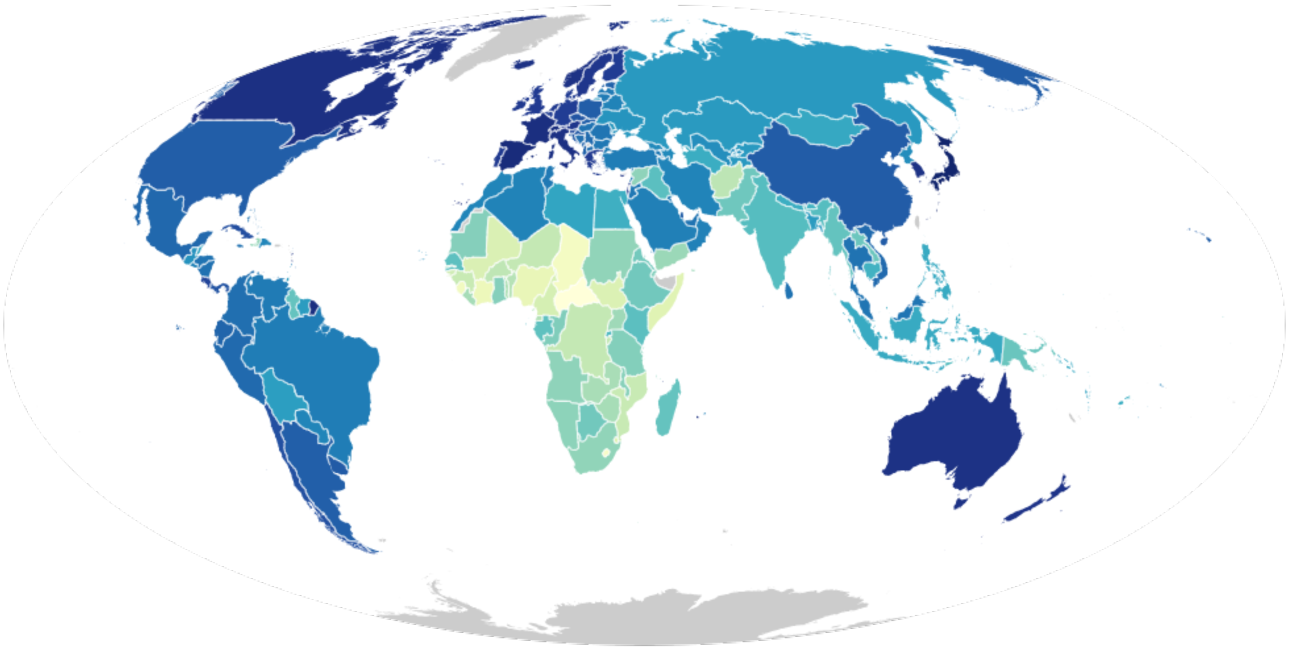

Figure 40: Map 2 of P20. Projection: Mollweide.
