# Supplementary material for: Mapping the Global South: Equal-Area Projections for Choropleth Maps
Source: arXiv:2008.13592 ancillary file (2020-09-06)
Supplement: Supplementary file 2 [file survey.pdf]

# Supplemental Material: Survey

Welcome to our survey!

This survey is meant to investigate what is important on the process of designing choropleth world maps. The results are anonymized. We will use them for designing (<system name anonymized>) maps and for our ongoing research. Completing the survey takes around 20 minutes.

## 1 YOUR MAP

This first section is about designing maps for your personal research.

1. Please shortly describe your research goals (e.g., what kind of research questions are you interested in?).

---

2. Are you interested in a specific world region or country?

   [ ] Yes

   [ ] No

3. In which world region or country are you interested in?

---

   {Question shown if the answer above was "Yes"}

4. We would like you to create a world map visualizing example data. You can find the task here:

   Task 1

   (link to notebook)

   When you are done, please download the map in the website using the "Save map 1" button and upload it here in the survey below without changing the file name.

   The task link takes you to Observable, a computational notebook for visualizations. We log the interactions anonymously through Google Analytics.

   (Upload button)

5. Please rank the 4 parameters based on how important they were for you to design your map (most important on top):

   - Map projection
   - Horizontal rotation
   - Color palette
   - Level of detail (zooming and panning)

   You need to drag and drop each element from the left box to the right box.

6. Please explain the reasoning behind your ranking shortly (e.g., why are some parameters more important for you than others?)

---

## 2 OUR MAP

This section is about designing a map for the research of the whole CRC.

1. We would like you to create a second world map according to the **goals of the CRC project**. The details of the goals are described in the task.

   You can find the task here:

   Task 2

   (link to notebook)

   When you are done, please download the map in the website using the "Save map 2" button and upload it here in the survey below without changing the file name.

   The task link takes you to Observable, a computational notebook for visualizations. We log the interactions anonymously through Google Analytics.

   (Upload button)

2. Please rank the 4 parameters based on how important they were for you to design this map:

   - Map projection
   - Horizontal rotation
   - Color palette
   - Level of detail (zooming and panning)

   You need to drag and drop each element from the left box to the right box.

3. Please explain the reasoning behind your ranking shortly (e.g., why are some parameters more important for you than others?).

---

## 3 DEMOGRAPHICS

1. Please rate your level of knowledge of cartography.

   Very limited [1] [2] [3] [4] [5] Very good

2. Do you work at the CRC 1342: Global Dynamics of Social Policy?

   [ ] Yes

   [ ] No

3. Please indicate your gender.

   [ ] Male

   [ ] Female

   [ ] Other

4. (Optional:) Please indicate your age.

5. (Optional:) Could we contact you in the future to get more feedback about this topic?

   If yes, please indicate your e-mail below.

6. (Optional:) Do you have any final comments or remarks?
